# Supplementary material for: Visuo-Tactile based Predictive Cross Modal Perception for Object Exploration in Robotics
Source: arXiv:2405.12634 source file (2024-05-23)
Supplement: Supplementary file 1 [file appendix.tex]

\section*{Appendix}
We also present the qualitative results of all the distint shapes in the object list estimated via the superquadric approach. 

\begin{figure}[h]
    \centering
    \includegraphics[width = \columnwidth]{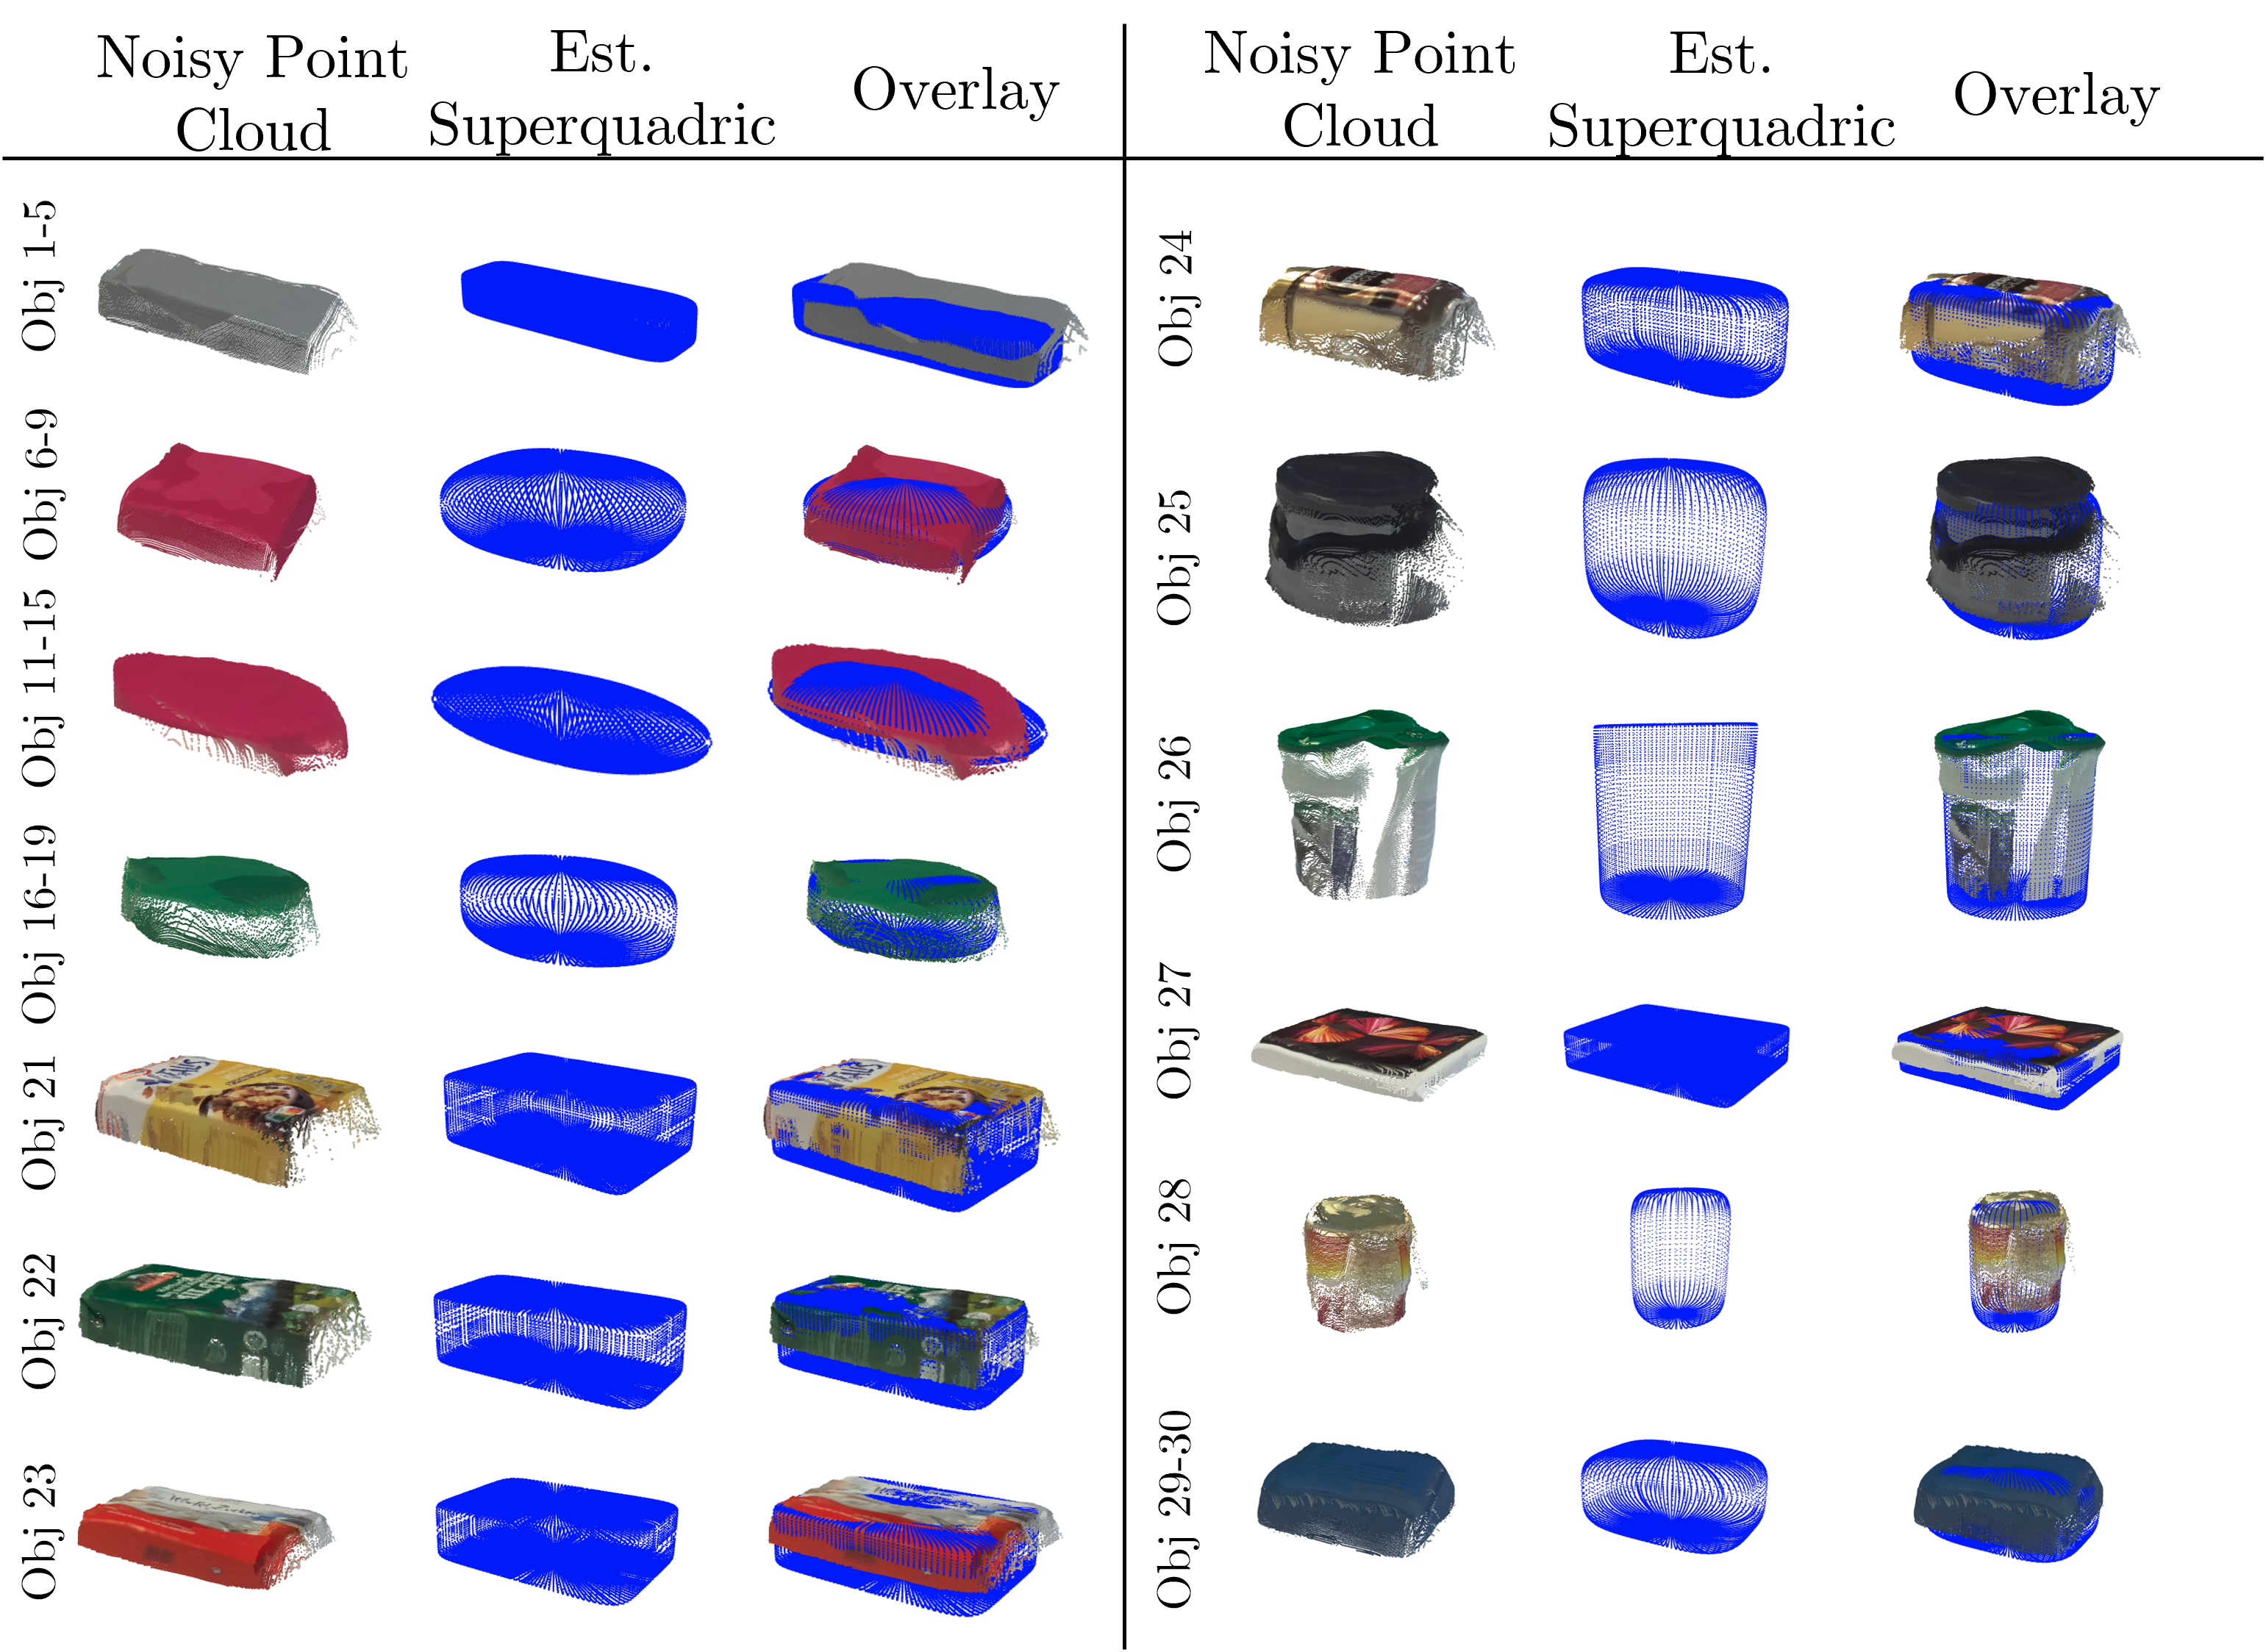}
    \caption{Qualitative Shape Results (to be updated)}
    \label{fig:qual_shape}
\end{figure}
